# Supplementary material for: On Privatizing Equilibrium Computation in Aggregate Games over Networks
Source: arXiv:1912.06296 source file (2019-12-13)
Supplement: Supplementary file 1 [file appendix_a.tex]

%!TEX root = root.tex

\section{Proof of Lemma~\ref{Lem:errors.converge}}
Let $T^k_i = x^{k}_i - x^{k-1}_i$ and we observe,
\begin{small}
\begin{align}
    y^k &= y^0 + \sum_{s=1}^k \left( y^s - y^{s-1} \right) = \frac{1}{N} \left( \sum_{i=1}^N v^0_i + \sum_{s=1}^k \sum_{j=1}^N T^s_j \right). \label{Eq:Lemma4Proof1}%
\end{align}%
\end{small}%
The second equality follows form Lemma~\ref{Lem:AggregateInvariance}.

Next, we build a expression for $\hat{v}^k_j$ using the aggregate update relation. Let $\mathcal{H}^s_i = \sum_{j=1}^N W_{ij}r^s_{ji}$.  

\begin{small}
\begin{align}
    &v^{k+1}_i = \hat{v}^k_i + x^{k+1}_i - x^k_i = \sum_{j=1}^N W_{ij} ( v^k_{j} + \alpha_k r^k_{ji} ) + T^{k+1}_i\nonumber \\
%    &= \sum_{j=1}^N W^k[i,j] v^k_{ji} + T^{k+1}_i \nonumber \\
%    & \nonumber \\
    &= \sum_{j=1}^N W_{ij} v^k_{j} +  \alpha_k \mathcal{H}^k_i + T^{k+1}_i \nonumber \\
%    &= \sum_{j=1}^N W_{ij} (\sum_{l=1}^N W_{jl} v^{k-1}_{l} + \alpha_{k-1} H^{k-1}_j + T^{k}_j) + \alpha_k \mathcal{H}^k_i + T^{k+1}_i \nonumber \\
     &= \sum_{l=1}^N W^2_{il} v^{k-1}_l  + \sum_{j=1}^N W_{ij} T^k_j + \alpha_k \sum_{j=1}^N W_{ij} H^{k-1}_j + \alpha_k \mathcal{H}^k_i + T^{k+1}_i \nonumber \\
     &\qquad \qquad \ldots \nonumber \\
     &= \sum_{l=1}^N W^{k+1}_{il} v^{0}_l  + \sum_{s=1}^k \sum_{j=1}^N W^{k-s+1}_{ij} T^s_j \nonumber \\
    &\qquad + \sum_{s=1}^k \alpha_{s-1} \sum_{j=1}^N W^{k-s+1}_{ij} \mathcal{H}^s_j + \alpha_k \mathcal{H}^k_i +  T^{k+1}_i. \label{Eq:Lemma4Proof2}
\end{align}
\end{small}

\noindent Moreover, observe that $\sum_{j=1}^N \mathcal{H}^k_j = \sum_{j=1}^N \sum_{l=1}^N W_{jl} r^k_{lj}$. Since the non-zero weight (in $W_{ij}$) corresponding to edge $(i,j)$ is always $\delta$, we have, $\sum_{j=1}^N \sum_{l=1}^N W_{jl} r^k_{lj} = 0$, implying, $(1/N)\sum_{j=1}^N \mathcal{H}^k_j = 0$ for any $k$. Using this we rewrite Eq.~\eqref{Eq:Lemma4Proof2},
\begin{small}
\begin{align}
    &v^{k+1}_i = \sum_{l=1}^N W^{k+1}_{il} v^{0}_l  + \sum_{s=1}^k \sum_{j=1}^N W^{k-s+1}_{ij} T^s_j + T^{k+1}_i\nonumber \\
    &\qquad \qquad + \sum_{s=1}^k \alpha_{s-1} \sum_{j=1}^N \left(W^{k-s+1}_{ij} - \frac{1}{N}\right) \mathcal{H}^s_j + \alpha_k \mathcal{H}^k_i\nonumber \\
    &\hat{v}^k_i = v^{k+1}_i - T^{k+1}_i = \sum_{l=1}^N W^{k+1}_{il} v^{0}_l  + \sum_{s=1}^k \sum_{j=1}^N W^{k-s+1}_{ij} T^s_j \nonumber \\
    &\qquad  + \sum_{s=1}^k \alpha_{s-1} \sum_{j=1}^N \left(W^{k-s+1}_{ij} - \frac{1}{N}\right) \mathcal{H}^s_j + \alpha_k \mathcal{H}^k_i \label{Eq:Lemma4Proof3}
\end{align}
\end{small} 

\noindent Observe that, $\|T^s_i\| = \|x^s_i - x^{s-1}_i\|$ is bounded as follows,
\begin{align*}
    \|T^s_i\| &= \|\mathcal{P}_{\mathcal{X}_i}[x^{s-1}_i - \alpha_{s-1} \nabla_{x_i} f_i(x^{s-1}_i, N \hat{v}^{s-1}_i)] - x^{s-1}_i\| \nonumber \\
    &\leq \|x^{s-1}_i - \alpha_{s-1} \nabla_{x_i} f_i(x^{s-1}_i, N \hat{v}^{s-1}_i) - x^{s-1}_i\| \nonumber \\
    &\leq \alpha_{s-1} C.   \qquad \qquad \qquad \qquad \qquad \qquad \text{(see Lemma~\ref{Lem:GradientBound})}
\end{align*}
And, $\|H^k_i\| = \|\sum_{j=1}^N W_{ij} r^k_{ji}\| \leq \|\Delta\|$ since $W$ is row stochastic and $\|r^k_{ji}\| \leq \Delta$

\noindent We subtract Eq.\eqref{Eq:Lemma4Proof3} from Eq.\eqref{Eq:Lemma4Proof1}, to get,
\begin{small}
\begin{align*}
\|y^k - \hat{v}^k_i\| &=  \sum_{l=1}^N \| W^k_{il} - \frac{1}{N} \| \|v^{0}_l\| + \sum_{s=1}^k \sum_{j=1}^N \|W^{k-s+1}_{ij} - \frac{1}{N} \| \|T^s_j\| \nonumber \\
&\quad + \alpha_k \| \mathcal{H}^k_i \| + \sum_{s=1}^k \alpha_{s-1} \sum_{j=1}^N \|W^{k-s+1}_{ij} - \frac{1}{N}\| \|\mathcal{H}^s_j\|%
\end{align*}%
\end{small}%
\noindent and further use the geometric convergence of product of doubly stochastic transition matrices and the bounds on $\|T^s_j\|$ and $\|H^s_j\|$,
\begin{align*}
\|y^k - \hat{v}^k_i\| &=  \theta \beta^k M + \theta N (C + \Delta) \sum_{s=1}^k\beta^{k-s} \alpha_{s-1} + \Delta \alpha_k 
\end{align*}
where, $M = \max_{l \in \Ncal} \|v^0_l\|$.
